# Supplementary material for: Tackling the Accuracy-Interpretability Trade-off in a Hierarchy of Machine Learning Models for the Prediction of Extreme Heatwaves
Source: arXiv:2410.00984 source file (2025-03-28)
Supplement: Supplementary file 1 [file SupMat.pdf]

# Supplementary Materials for

## Tackling the Accuracy-Interpretability Trade-off in a Hierarchy of Machine Learning Models for the Prediction of Extreme Heatwaves

Alessandro Lovo, Amaury Lancelin, Corentin Herbert and Freddy Bouchet

Corresponding author: **Freddy Bouchet** ([freddy.bouchet@cnrs.fr](mailto:freddy.bouchet@cnrs.fr))

### Contents of this file

Text S1 to S5

Figures S1 to S15

## S.1 Pareto plots

For the interpretable models of the Gaussian approximation (GA) and Intrinsically Interpretable Neural Network (IINN), we have a visualizable projection pattern  $M$ . For  $M$  to be interpretable, we require it to be spatially smooth, by adding a regularization term to the loss function. As explained in Mascolo et al. (2024), this can be achieved either penalizing directly the roughness  $H_2$  of the projection pattern (solid lines in figs. S1 and S2) or indirectly penalizing its  $L_2$  norm (dashed lines in figs. S1 and S2). In any case, we need to find the proper value of the regularization coefficient,  $\epsilon$  which gives a good compromise between skill and interpretability. Since there are two objectives to optimize at the same time, we call the plots in figs. S1 and S2 Pareto plots.

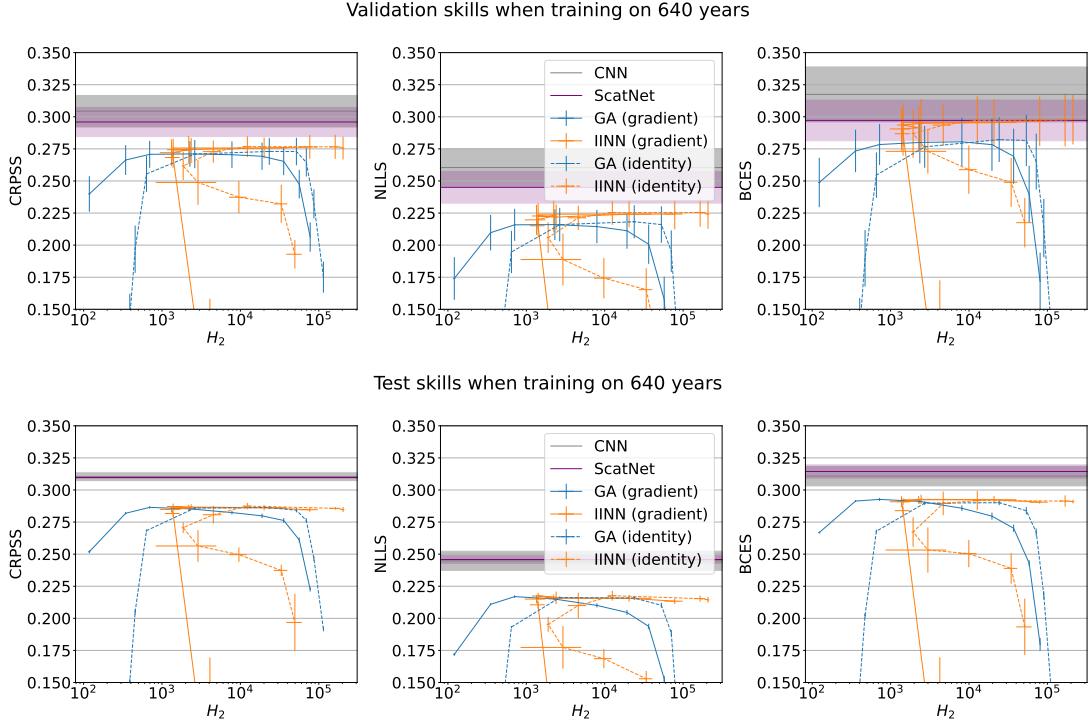

Figure S1: Pareto plots when training on the 640-year-long datasets. Skill on the y-axis (higher is better) for the three metrics, and roughness ( $H_2$ ) of the projection pattern on the x-axis (lower is better). CNN and ScatNet don't have a projection pattern, so we report their skill as constant across values of  $H_2$ . For IINN and GA, we show the results both with L2 regularization (identity) and gradient regularization (gradient). The latter gives better results and is the one used in the main text of this paper. For validation, the error bars and shading correspond to the 5 different models being evaluated on the 5 different 160-year-long validation sets. For test, the error bars and shading are due only to the 5 different models being evaluated on the common 200-year-long test set.

Focusing on the top row of fig. S1, we see that both IINN and GA, for both types of regularization, have a broad plateau of good skill, with performance drops on both sides. On the right side,  $\epsilon$  is very small, and thus the pattern is very rough. For GA (blue curves), this severely impacts the validation performance, as the model is overfitted to the training data. On the other

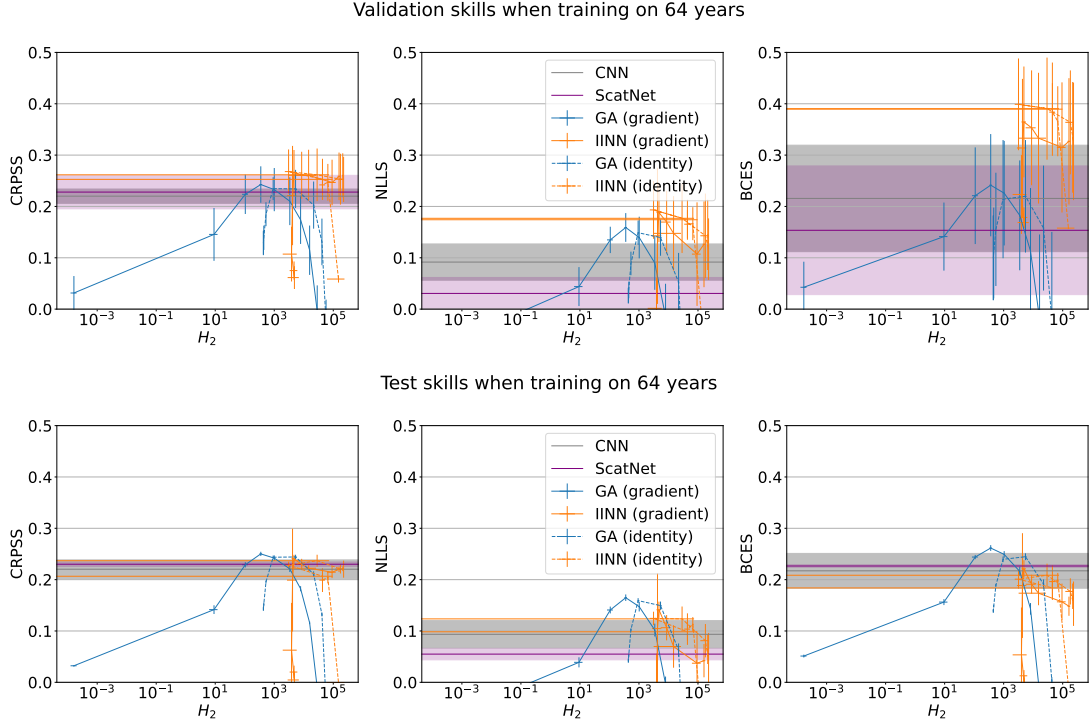

Figure S2: Same as fig. S1, but when training on the smaller 64-year datasets

hand, IINN (orange curves) can somewhat compensate overfitting with the network following the linear projection, namely by predicting a higher variance. More interesting is the behavior on the left side. Again, for GA, the pattern is now too smooth and so the model isn't flexible enough to capture the important information. IINN, however, has a weird behavior, where increasing too much the regularization coefficient leads to rougher patterns (the curves bend back towards the right). This is simply explained by the fact that while GA is trained in one step (Mascolo et al., 2024), IINN is optimized with gradient descent starting from randomly initialized weights. Since we use an early stopping protocol on the validation skill to avoid overfitting, when  $\epsilon$  is too high, the main evolution of the pattern is to make it smooth rather than predictive. This means that early stopping kicks in too early and the model is checkpointed back to one of the early epochs where the projection pattern was still very rough.

By comparing the two types of regularization, we can see that  $L_2$  regularization yields slightly higher validation skills. However, the Pareto optimum is to be as close as possible to the top left corner of the plot (high skill, low roughness), and thus we choose to use  $H_2$  regularization.

The second row of fig. S1 shows the Pareto plots when the metrics are evaluated on the test set. Any skill gain that more complex (IINN with respect to GA) or less regularized architectures had in the validation set is completely lost on the test set. This suggests that these marginal gains were effects of overfitting on the validation set during the hyperparameter optimization phase.

In fig. S2, we display the same results for the networks trained on the shorter 64-year-long datasets. The conclusions about IINN and GA are very similar to the ones for the longer dataset, and the main difference is the greatly reduced performance of CNN and ScatNet, which

now display the worst skills in the hierarchy.

## S.2 CNN : Local Interpretability

In fig. 4 of the main text, we show several examples of local feature importance maps with Expected Gradients (EGFI). For visual purposes, we chose to smooth these maps by a Gaussian filter with  $\sigma = 1.3$  pixels. We also normalize the maps by the sum of feature importance (that is equal to  $\hat{\mu}$  according to the completeness axiom (Sundararajan et al., 2017)) to have a better visual comparison between different predictions. In fig. S3, we show an example of a raw EGFI map (middle) and its Gaussian-smoothed version (right).

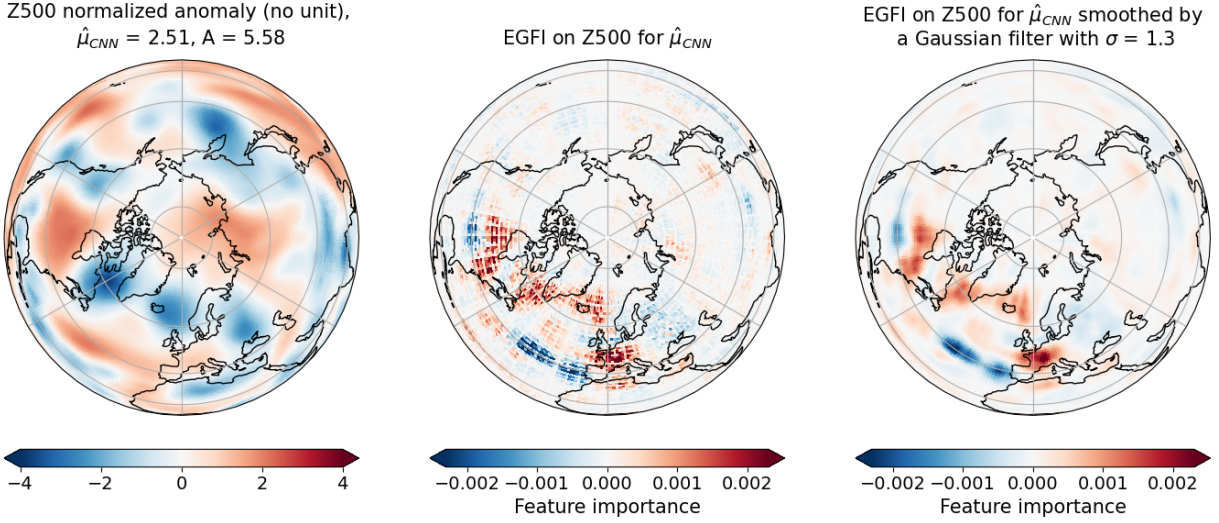

Figure S3: raw Expected Gradients feature importance (EGFI) (middle) and Gaussian-smoothed EGFI (right) for the prediction of  $\hat{\mu}(X)$  with the CNN. The smoothing helps in highlighting the broader areas of influence with less noise. For the Gaussian filter, we set  $\sigma = 1.3$  on qualitative grounds. We also show the corresponding Z500 input (left) from the test set, selected from the heatwaves example. We show, among the 5 CNN models, the one with the highest skill.

As shown in fig. 4 of the main text, the EGFI maps exhibit a strong correlation with the GA projection pattern multiplied by the input (third row). To quantify this relationship more systematically, we compute the pattern correlation between the EGFI maps and the GA projection pattern multiplied by the input for each test set sample. This correlation is measured using a normalized dot product, accounting for the different area of each pixel. The histogram of these correlation coefficients (each between -1 and 1) is presented in fig. S4, demonstrating that the EGFI maps are highly correlated with the GA maps, with a mean correlation of 0.84 and a standard deviation of 0.08.

In fig. 2 of the main text, we show the EGFI maps for the prediction of  $\hat{\mu}(X)$  with the CNN only for Z500. In fig. S5, we complement this figure by showing the EGFI maps for the soil moisture input. Also, as done in the main text, we show the point-wise multiplication between the input and the GA projection pattern, which amounts to computing the EGFI for the GA

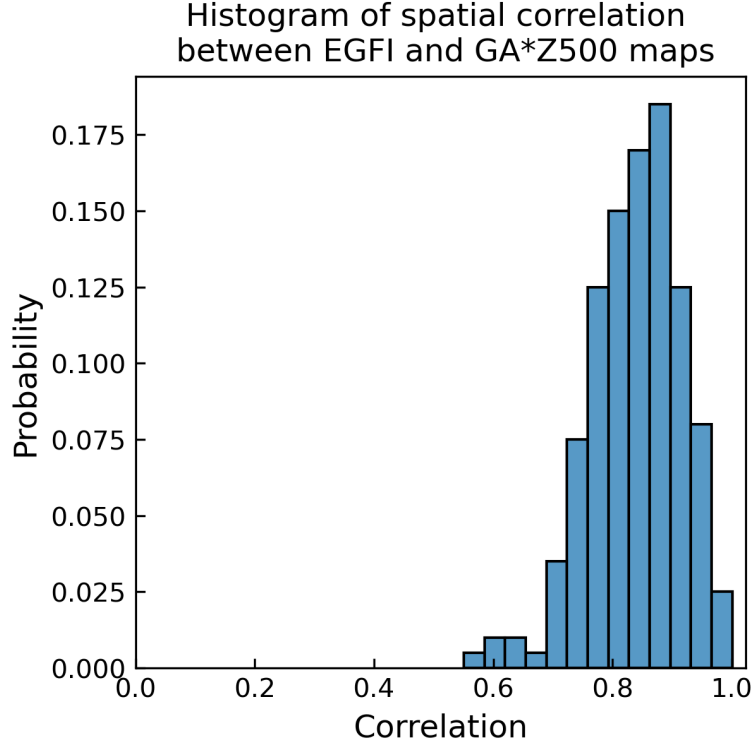

Figure S4: Histogram of the pattern correlation between the EGFI maps and the GA projection pattern multiplied by the input for inputs of the test set. The mean correlation is 0.84 and the standard deviation is 0.08. The correlation is computed using a normalized dot product.

prediction. We can see that the GA projection pattern is very smooth and has a clear spatial structure. The EGFI maps for the CNN prediction show a quite similar structure, but with a large amount of noise.

Finally, as our models predict both the mean and the standard deviation of the heatwave amplitude, we can also compute the EGFI for the standard deviation. Figure S6 presents the EGFI maps of Z500 for predicting  $\hat{\sigma}(X)$  using the CNN. The EGFI maps exhibit significant noise. Notably, for specific inputs, such as the first two on the left in the top row, a structure far from France, located in the Northeastern United States, significantly influences the predicted standard deviation. This teleconnection indicates that strong positive anomalies in the geopotential height in the Northeastern United States are linked to higher uncertainty in predicting the heatwave amplitude in France. This connection seems reasonable, given the eastward propagation of weather patterns.

### S.3 CNN: Optimal input

In fig. S7 we show the effect of direct backward optimization of  $\hat{\mu}_{\text{CNN}}$  on a sample point from the test data. Such optimization follows the complex non-linearities of the CNN and thus leads to a very rough optimized input, and an extremely unrealistic predicted heatwave amplitude of 36 K. To counteract this effect and have more physically realistic maps, we add to the simple

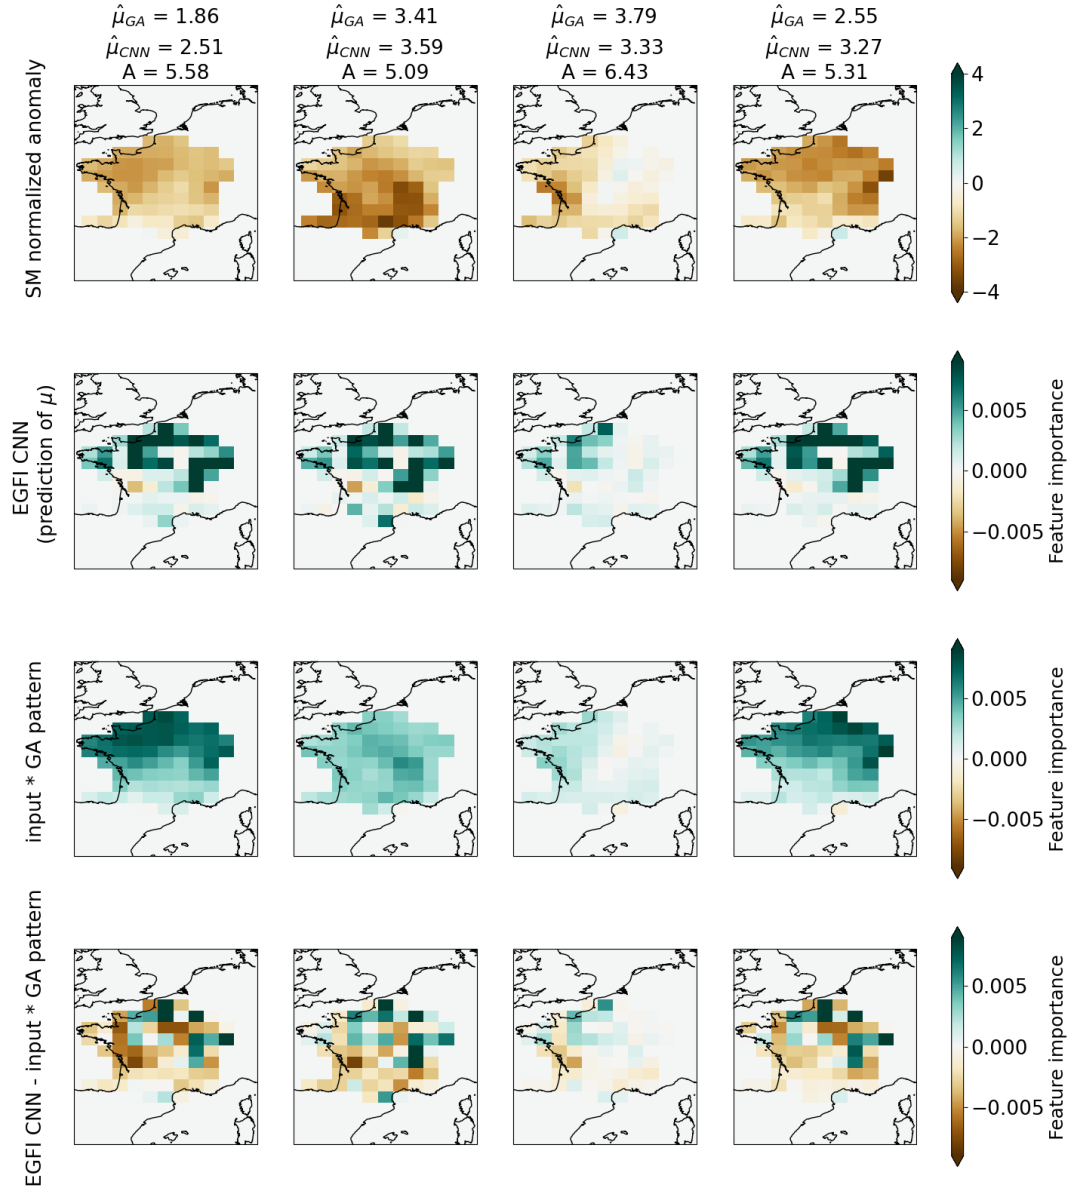

Figure S5: Top row: Several normalized soil moisture initial conditions  $X$  (inputs) associated with  $A$  above the 95<sup>th</sup> percentile (heatwaves). Second row: Expected Gradients feature importance (EGFI) on soil moisture of the CNN predictions. Third row: point-wise multiplication between inputs and GA projection pattern. Since  $\hat{\mu}_{GA}(X)$  is linear in  $X$ , this amounts to compute EGFI for the GA prediction. Fourth row: EGFI CNN minus EGFI GA for each input. We show, among the 5 models, the one with the highest skill. Here, the EFGI maps are not smoothed by a Gaussian filter.

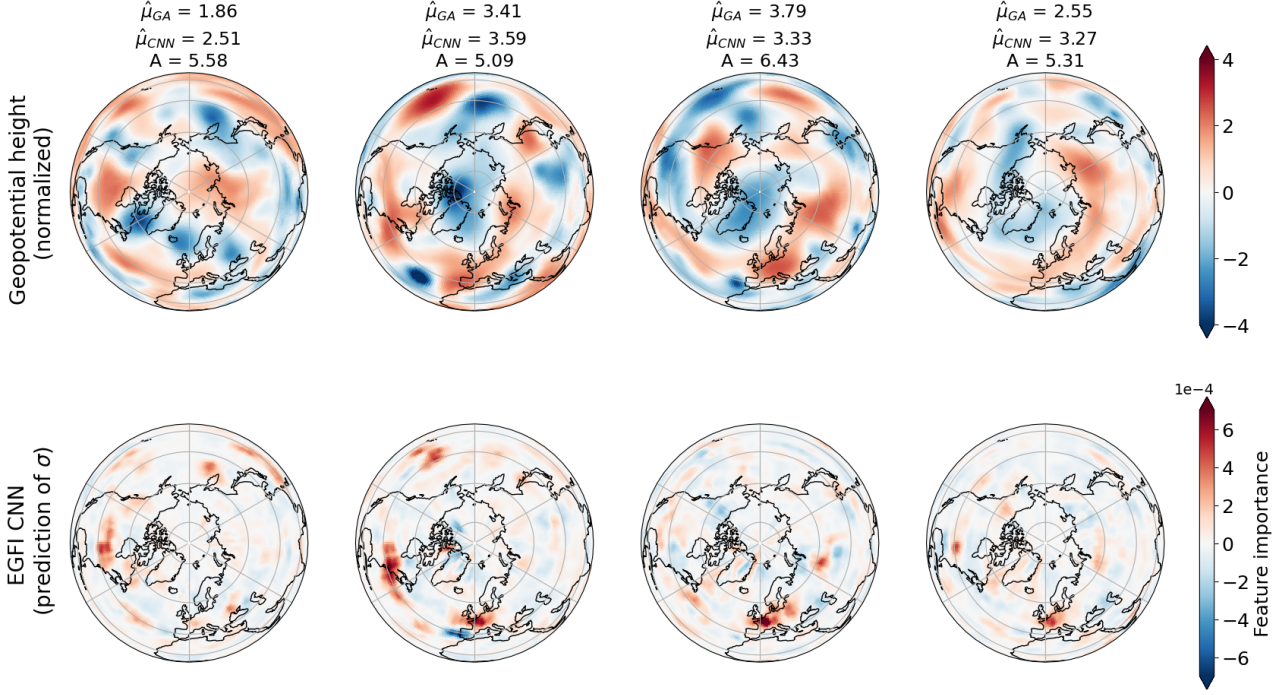

Figure S6: Top row: Several normalized Z500 initial conditions  $X$  (inputs) associated with  $A$  above the 5th percentile (heatwaves). Second row: Expected Gradients feature importance (EGFI) on Z500 of the CNN predictions of  $\hat{\sigma}(X)$ . We show, among the 5 models, the one with the highest skill.

loss  $\ell = -\hat{\mu}_{CNN}(S)$  terms constraining the roughness and  $L_2$  norm of  $S$ . In particular, when we plot the histogram of these quantities for test data, we find that the distributions are relatively narrow (fig. S8). Then, we modify the loss  $\ell$  as

$$\ell = -\hat{\mu}_{CNN}(S) + \lambda_2 (|S| - n_0)^2 + \lambda_r \left( \sqrt{H_2(S)} - r_0 \right)^2, \quad (\text{S6})$$

where  $n_0$  and  $r_0$  are respectively the average  $L_2$  norm and roughness of the test data, and  $\lambda_2$  and  $\lambda_r$  are the two regularization parameters.

To complement the information presented in the main text about the average optimal input, we present in figs. S9 and S10 the distribution of the predicted heatwave amplitude. From fig. S9 we can see that, despite having imposed some physical constraint in the form of roughness and  $L_2$  norm, the distribution of the predicted heatwave amplitude (orange) is still very far from the actual heatwave events in the test data (blue). We also see that the predicted heatwave amplitude mainly consists of the Gaussian component  $\hat{\mu}_{GA}$ , with the non-linear part  $\hat{\mu}_{pert} = \hat{\mu}_{CNN} - \hat{\mu}_{GA}$  (green) accounting only for a sixth of the predicted heatwave amplitude.

Forcing the optimization to move orthogonally to the Gaussian approximation projection pattern (fig. S10) yields lower predicted values. From this latter plot we can see that the variance of  $\hat{\mu}_{CNN}$  is much higher with respect to the previous plot, but this is due to the fact that moving orthogonally to the projection pattern leads  $\hat{\mu}_{GA}$  to stay constant during the optimization, and thus retain the distribution it had for the prediction on test data. Indeed,  $\hat{\mu}_{pert}$ , which is what is freely optimized, retains a similar variance to the one it had in the previous plot.

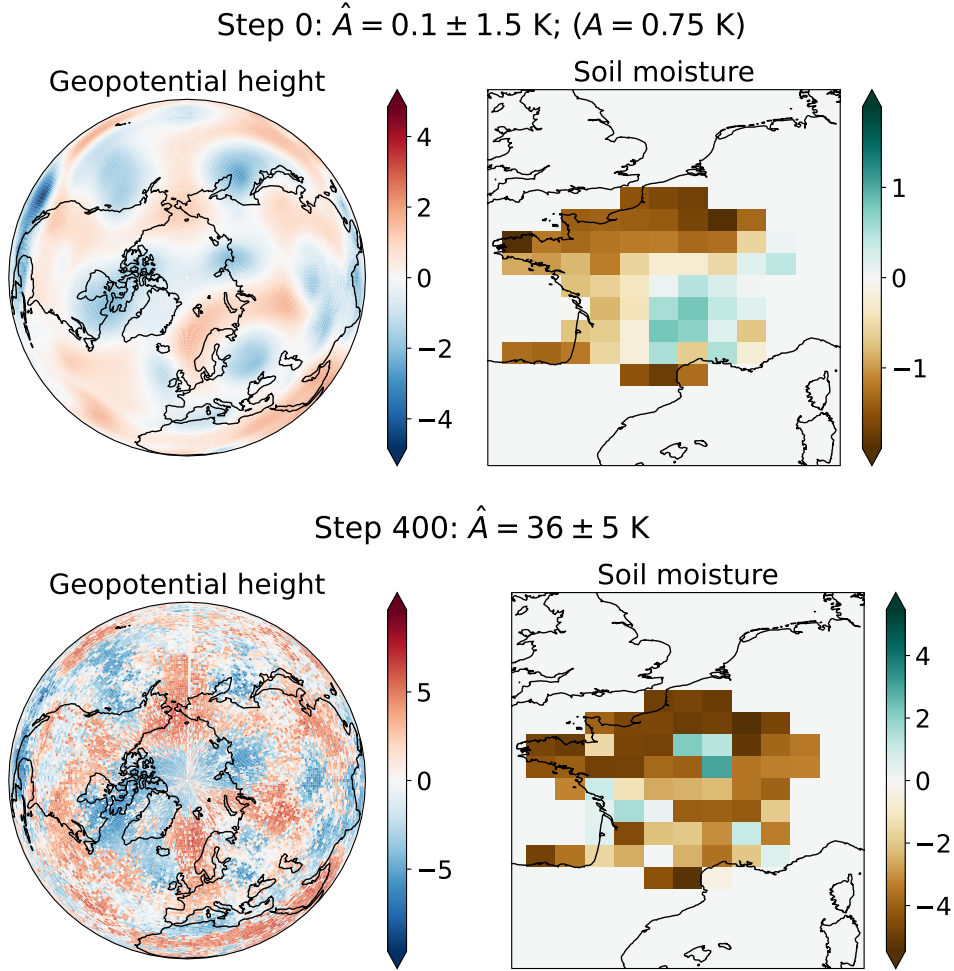

Figure S7: Example of the effect of the unconstrained backward optimization of  $\hat{\mu}_{\text{CNN}}$  on a typical snapshot from the test set (top), after 400 iterations of gradient descent (bottom). For both figure we report the prediction of the CNN and for the first also the true value of the heatwave amplitude  $A$ .

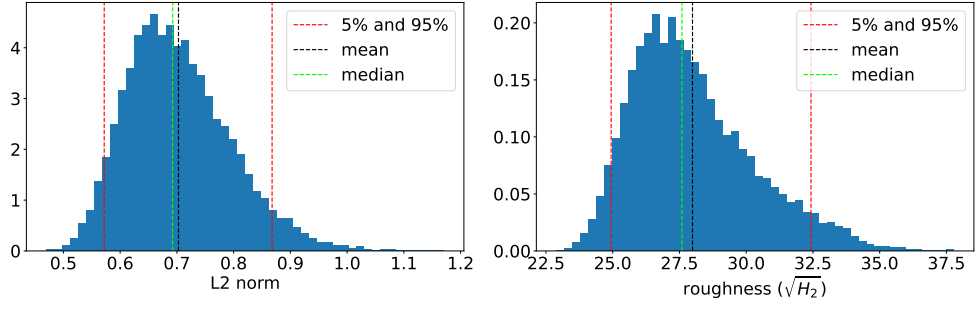

Figure S8: Histograms of the  $L_2$  and  $H_2$  norms of the test data. Vertical lines show the mean, median and 5% and 95% quantiles

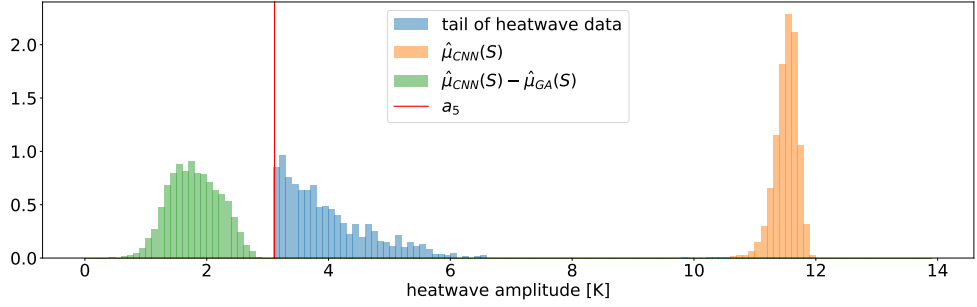

Figure S9: Histograms of the heatwave amplitude in the tail (5% most extreme events) of the distribution of test data (blue), of the mean heatwave amplitude  $\hat{\mu}_{\text{CNN}}(S)$  predicted by the CNN on the optimized inputs  $S$  (orange) and of the difference between the prediction of CNN and GA (green).

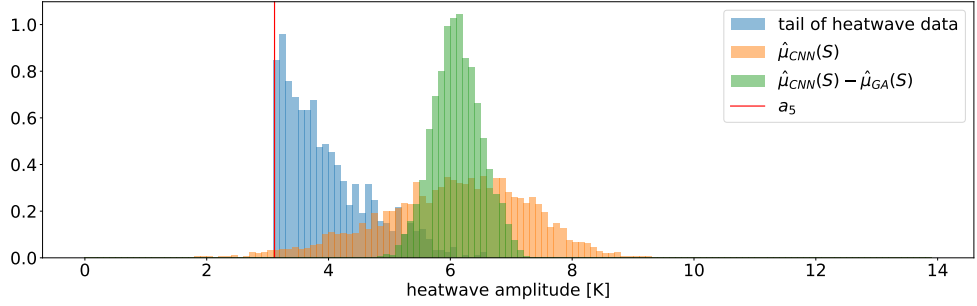

Figure S10: Histograms of the heatwave amplitude in the tail (5% most extreme events) of the distribution of test data (blue) and of the mean heatwave amplitude  $\hat{\mu}_{\text{CNN}}(S)$  predicted by the CNN on the optimized inputs  $S$  in an orthogonal direction to the projection pattern of the Gaussian approximation (orange). In green, the difference between the prediction of CNN and GA, where the latter didn't change during the optimization process.

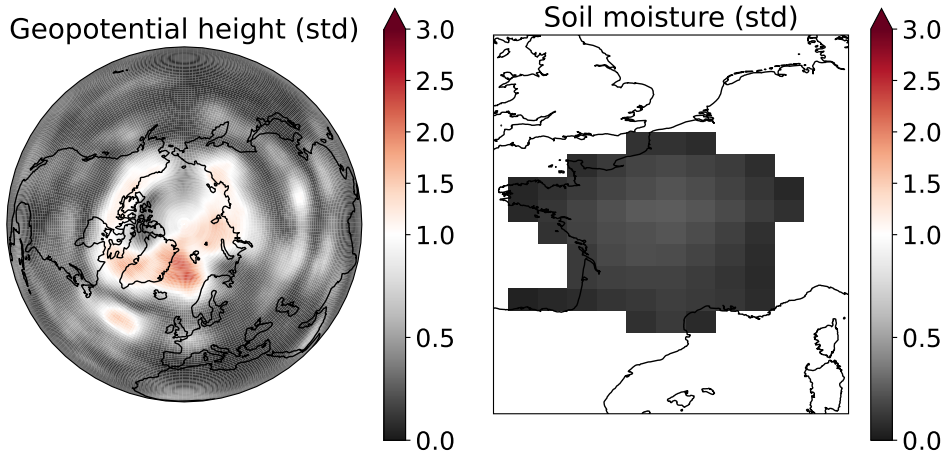

Figure S11: Map of the standard deviation of the optimized inputs  $S$  that maximize the heatwave amplitude  $\hat{\mu}_{\text{CNN}}(S)$  predicted by the CNN, across the different seeds  $S_0$  taken from the test dataset.

In figs. S11 and S12, we show the maps of standard deviation of the optimized inputs, respectively without and with the orthogonality constraint. Since the original inputs have a pixel-wise standard deviation of 1, we color in gray regions where the optimization concentrates the data and in red regions where instead the original variance is amplified.

The second row of figs. 2 and 3 of the main text is obtained as the pixelwise ratio between their first row and figs. S11 and S12 respectively.

#### S.4 Scatnet

In fig. S13, we present the feature importance of first-order features for the prediction of  $\hat{\mu}(X)$  using ScatNet across various scales and for orientation  $\theta = 0$ . For any given orientation  $\theta$ , the feature importance maps are proportional across scales, with a reduced amplitude for smaller scales  $j$ . This proportional behavior is consistent across other orientations, though not depicted here.

The question arises as to why these maps are proportional. Initially, it is not apparent that the model should learn identical patterns at different scales, as there are no intrinsic reasons for this. However, considering that wavelet filters are non-local in the frequency domain and their supports overlap, we expect these patterns to be close in some way, either in spatial pattern or amplitude (or both combined).

In fig. 6 of the main text, we observed that as we transition between orientations, the spatial pattern of feature importance changes continuously. Here we observed, when transitioning from a larger scale  $j$  to a smaller one, that the spatial pattern remains the same but with diminished amplitude. Although we do not have a clear explanation for these behaviors, we interpret them as indications of robustness, as the model does not appear to be learning mere noise.

Additionally, we observed the robustness of feature importance maps across each indepen-

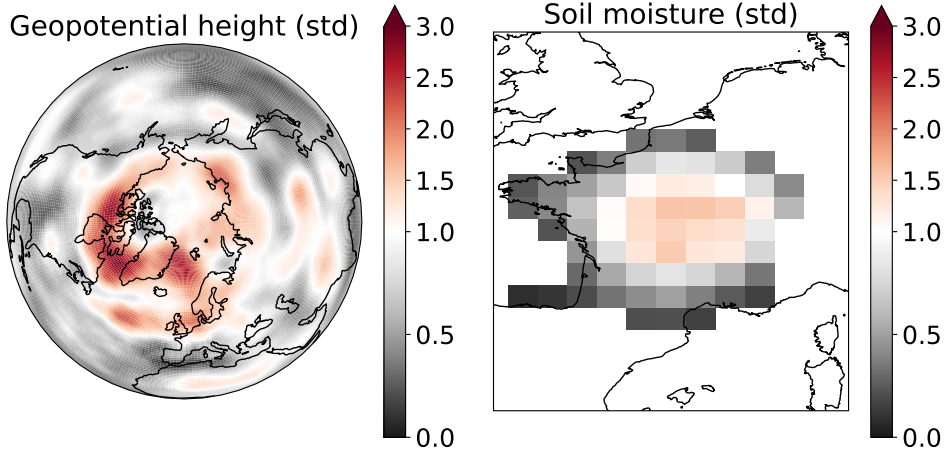

Figure S12: Map of the standard deviation of the optimized inputs  $S$  that maximize the heatwave amplitude  $\hat{\mu}_{\text{CNN}}(S)$  predicted by the CNN while keeping fixed the prediction  $\hat{\mu}_{\text{GA}}(S)$  of the Gaussian approximation, across the different seeds  $S_0$  taken from the test dataset.

dent model used in the 5-fold cross-validation (not shown here), further supporting the model's reliability.

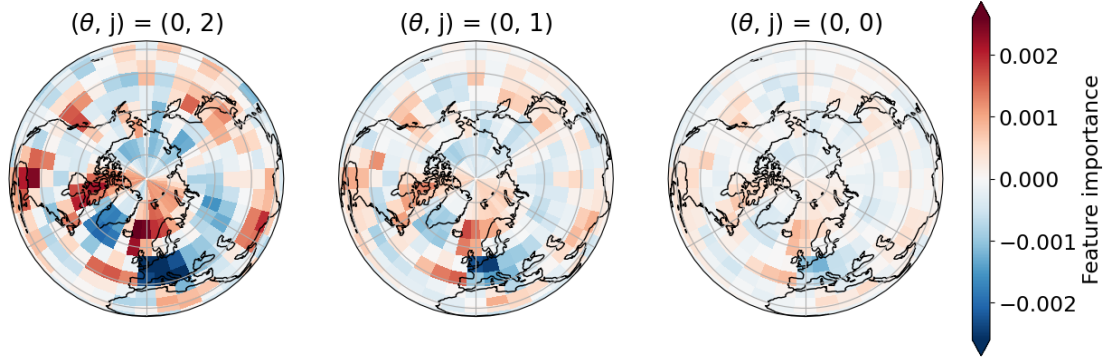

Figure S13: Feature importance of first order features for the prediction of  $\hat{\mu}(X)$  on 500-hPa geopotential height with ScatNet for each scale and for orientation  $\theta = 0$ . For any given orientation  $\theta$ , the feature importance maps at different scales  $j$  are proportional, but with less amplitude for smaller scales. See fig. 6 of the main text for maps at different orientations for  $j = 2$ . We show here the average maps across the 5 models.

In addition to the previous analysis, we investigate the question of how much information is lost when reconstructing the input from the scattering coefficients. Figure S14 presents the reconstruction of the input from the scattering coefficients for zero and first order features, which are used for the prediction of  $\hat{\mu}(X)$ . These maps are obtained by inverting the ScatNet transform by using a gradient-ascent algorithm.

The reconstruction is not perfect, but it is remarkably accurate. The zero order scattering coefficients ensure that the precise location of cyclones and anticyclones is preserved, as these structures are larger than the coarsening scale of  $2^3$  pixels. Furthermore, the reconstruction also captures finer scale details present in the original input. However, it appears that the reconstruction for the smallest scales introduces structures that are not present in the original input: a form of "hallucination".

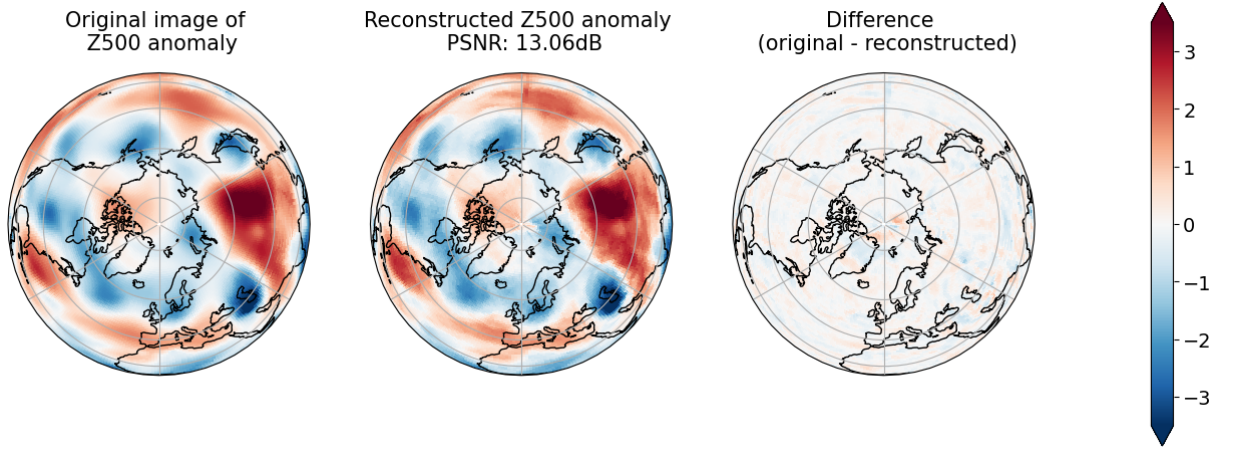

Figure S14: Reconstruction of a Z500 anomaly input from the scattering coefficients for zero and first order features. The first column shows the original Z500 anomaly input, the second column shows the reconstruction from the scattering coefficients, and the third column shows the difference between the original input and the reconstruction. We invert the scattering transform by using a gradient-ascent algorithm.

## S.5 Data normalization

The input data that we feed to the neural networks is normalized such that each scalar predictor, i.e. each grid point of the two fields of 500 hPa geopotential height anomaly and soil moisture anomaly, has zero mean and unitary standard deviation.

To avoid contamination between training, validation and test sets, for each fold we use only the raw (i.e. non-normalized) training data  $\tilde{X}_{\text{train}}$  to compute the maps of pixel-wise mean  $\mu_X^{\text{train}}$  and standard deviation  $\sigma_X^{\text{train}}$ . We then use these maps to normalize training, validation and test sets.

$$X_{\text{train}} = \frac{\tilde{X}_{\text{train}} - \mu_X^{\text{train}}}{\sigma_X^{\text{train}}} \quad X_{\text{val}} = \frac{\tilde{X}_{\text{val}} - \mu_X^{\text{train}}}{\sigma_X^{\text{train}}} \quad X_{\text{test}} = \frac{\tilde{X}_{\text{test}} - \mu_X^{\text{train}}}{\sigma_X^{\text{train}}} \quad (\text{S14})$$

Since the raw data already consists of anomalies, and each training set contains 640 years out of the total 1000 years of available data, the mean  $\mu_X^{\text{train}}$  is close to zero everywhere (not shown). On the other hand, in fig. S15 we show the map of  $\sigma_X^{\text{train}}$ , which displays higher variance in the geopotential height field the closer we are to the pole. Soil moisture instead has higher fluctuations in the South-Eastern part of France, which has a more continental climate with respect to the North-West.

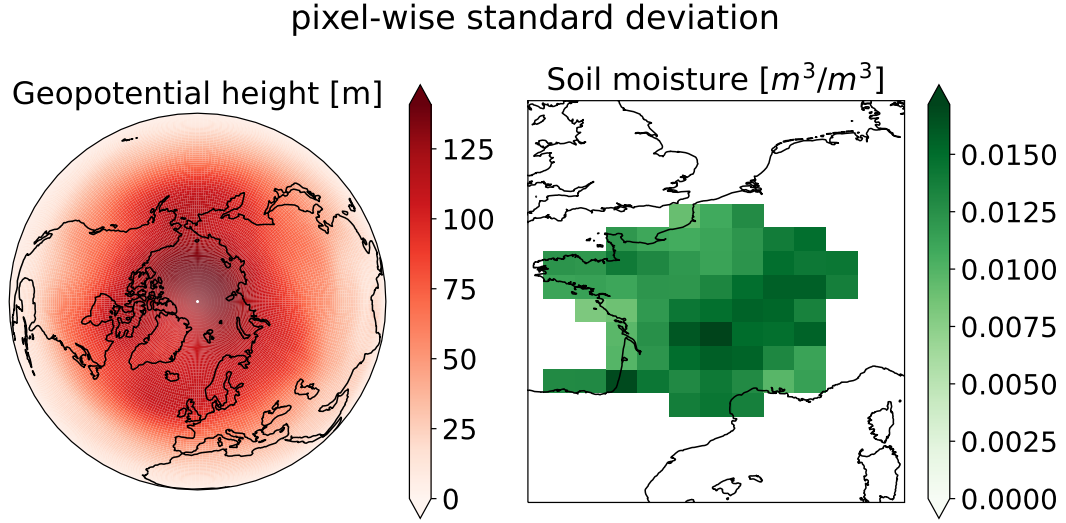

Figure S15: Map of the pixel-wise standard deviation  $\sigma_X^{\text{train}}$  of the input data before normalization, for the first fold. The maps for the other four folds are virtually identical.

## References

- Mascolo, V., A. Lovo, C. Herbert, and F. Bouchet, 2024: arXiv:2405.20903. Gaussian Framework and Optimal Projection of Weather Fields for Prediction of Extreme Events. arXiv.
- Sundararajan, M., A. Taly, and Q. Yan, 2017: Axiomatic attribution for deep networks. *International conference on machine learning*, PMLR, 3319–3328.
